# Supplementary material for: Efficient reduction of Kappa models by static inspection of the rule-set
Source: arXiv:1501.00440 source file (2015-01-02)
Supplement: Supplementary file 1 [file main_appendix.tex]

% This is LLNCS.DEM the demonstration file of
% the LaTeX macro package from Springer-Verlag
% for Lecture Notes in Computer Science,
% version 2.4 for LaTeX2e as of 16. April 2010
%
\documentclass{llncs}
\usepackage{makeidx}  % allows for indexgeneration
\usepackage{amsfonts,epsfig,graphicx,enumitem,multicol} 
\usepackage{amsmath}
\usepackage{amssymb} 
\usepackage{mathrsfs}
\usepackage[lined,linesnumbered]%boxed
{algorithm2e}
\usepackage{verbatim} 
\usepackage{epic}
\usepackage{eepic}
\usepackage{latexsym}
\usepackage{graphicx}
\usepackage{amsmath}
\usepackage{extarrows}
\usepackage{chemarr}

\begin{document}
\frontmatter          % for the preliminariesal
\pagestyle{headings}  % switches on printing of running heads
%\addtocmark{Hamiltonian Mechanics} % additional mark in the TOC
%
%
\mainmatter              % start of the contributions
\title{Prototyping genetic circuits with rule-based models: Appendix}
\titlerunning{Prototyping genetic circuits with rule-based models: Appendix}  % abbreviated title (for running head)
%                                     also used for the TOC unless
%                                     \toctitle is used
%
\author{Andreea Beica\inst{1} \and Calin Guet\inst{2}
%\and Tom Henzinger\inst{2} 
\and Tatjana Petrov\inst{2}}
\authorrunning{Beica et al.} % abbreviated author list (for running head)
%
%%%% list of authors for the TOC (use if author list has to be modified)
%\tocauthor{Ivar Ekeland, Roger Temam, Jeffrey Dean, David Grove,
%Craig Chambers, Kim B. Bruce, and Elisa Bertino}
%
\institute{ENS Paris,
Rue d'Ulm 45,
75005 Paris,
France
%\\ \email{@},\\ WWW home page:
%\texttt{http://users/\homedir iekeland/web/welcome.html}
\and
IST Austria,
Am Campus 1,
Klosteneuburg, Austria}

\maketitle              % typeset the title of the contribution

\input{dfnsA.tex}

\begin{abstract}
When designing genetic circuits, the typical primitives used in major existing modelling formalisms 
are gene interaction graphs, where edges between genes denote either activation or inhibition relation. 
However, when designing experiments, it is important to be precise about the low-level mechanistic details to how each such relation is implemented. 
Rule-based modelling language Kappa allows to unambiguously specify the mechanistic details such as DNA binding sites, the dimerisation of the transcription factors, or co-operative binding. However, such a detailed model comes with complexity and computationally costly executions. We propose a general method for automatically reducing a rule-based model, by eliminating intermediate species and adjusting the rate constants accordingly. Our method consists of %scanning the rule-set while 
searching for those interaction patterns that are known to be amenable to equilibrium approximations (such as the Michaelis-Menten scheme). 
The approximate model is efficiently obtained by static analysis over the rule-set, and it represents a particular theoretical limit of the original one. 
 %the separation of time-scale separation arguments and  
The tool is implemented in OCaml, and it is tested on a detailed rule-based model of a $\lambda$-phage switch, which lists
$96$ rules and $16$ proteins. % and $61$ species. 
The approximate model has $11$ rules and $5$ proteins, and it %outputs the lysogeny probability comas the detailed model, and it 
provides a dramatic reduction in simulation time.
%\tanja{Andreea, please fill in the numbers in the last two sentences}
%The simulation time of the appro
% and a number of smaller GRN circuits.
%for prototyping genetic circuits,  and other details which are known to be important
%for the circuit to function robustly. 
%Then, we perform the
%quantitative analysis of such a model, with a goal to observe the known
%facts about its high-level behavior.
%The processes in biochemical network often happen at different time-scales. 
%Approximation of fast sub-networks can significantly accelerate the simulation time.
%In this paper, we present a method and a tool for automated reduction of stochastic rule-based models.
% (for example, gene inhibition is either
%due to abundance of another molecule compatible to the transcription
%factor, or due to that the binding sites in the promoter region are
%already occupied by another transcription factor). 
%Moreover, the low-level models are suitable for mathematical analysis, because their rates respect mass-action law.
\end{abstract}

\input{appendix.tex}

\end{document}
